# Supplementary material for: Realisation of the Brazil-nut effect in charged colloids without external driving
Source: arXiv:2208.11102 ancillary file (2023-08-18)
Supplement: Supplementary file 1 [file SI_brazil.pdf]

# Supporting Information for

## Realisation of the Brazil-nut effect in charged colloids without external driving

**Marjolein N. van der Linden, Jeffrey C. Everts, René van Roij, and Alfons van Blaaderen**

**E-mail: m.n.vanderlinden@utwente.nl, jeffrey.everts@fuw.edu.pl, r.vanroij@uu.nl, a.vanblaaderen@uu.nl**

### This PDF file includes:

Supporting text
Figs. S1 to S5
Table S1
Legends for Movies S1 to S2
SI References

### Other supporting materials for this manuscript include the following:

Movies S1 to S2

## Supporting Information Text

## Dependence of the Brazil-nut effect on the bulk charge ratio

**Table S1. Summary of the system parameters for the four binary systems.** We report, for each particle, the average diameter $\sigma$ as determined by static light scattering (SLS) or scanning electron microscopy (SEM), the type of fluorescent dye used to label the particle, whether the particle is locked or unlocked, and the dimensionless electrostatic surface potential $\beta e\psi_0$ as determined by electrophoresis ($T = 298$ K) and the charge on the particle $Z$, assuming a Debye screening length $\kappa^{-1} \approx 6\ \mu\mathrm{m}$; for each binary system, we give the mass ratio $m_\mathrm{L}/m_\mathrm{S}$, the charge ratio $Z_\mathrm{L}/Z_\mathrm{S}$ between the large and small particles, and indicate whether we observed the colloidal Brazil-nut effect (BN) for that system. Values preceded by $\sim$ are estimates; see text for details.

| Binary system | Particle | $\frac{\sigma}{\mu m}$ | Dye | Locked? | $\eta$ | $\beta e\psi_0$ | $\frac{Z}{10^2}$ | $\frac{m_\mathrm{L}}{m_\mathrm{S}}$ | $\frac{Z_\mathrm{L}}{Z_\mathrm{S}}$ | BN |
|---|---|---|---|---|---|---|---|---|---|---|
| 1 | U20<br>U16 | 1.98<br>1.58 | NBD<br>RITC | no<br>no | 0.02<br>0.02 | 3.3<br>3.9 | 2.9<br>2.4 | 2.0 | 1.2 | no |
| 2 | L20<br>U16 | 1.98<br>1.58 | NBD<br>RITC | yes<br>no | 0.018–0.011<br>0.02 | 4.2–5.1<br>3.9 | 4.6–6.9<br>2.4 | 2.0 | 1.9–2.8 | yes |
| 3 | U29<br>U13 | 2.87<br>1.30 | NBD<br>RITC | no<br>no | ∼0.02<br>∼0.02 | ∼3.6<br>∼3.6 | ∼6.7<br>∼1.4 | 11 | ∼4.7 | no |
| 4 | L29<br>U13 | 2.87<br>1.30 | NBD<br>RITC | yes<br>no | 0.006<br>∼0.02 | 3.8<br>∼3.6 | 9.0<br>∼1.4 | 11 | ∼6.4 | no |

We prepared four binary systems (Table S1) with different buoyant mass ratios $m_\mathrm{L}/m_\mathrm{S} = \sigma_\mathrm{L}^3/\sigma_\mathrm{S}^3$, where $\sigma_\mathrm{L}$ and $\sigma_\mathrm{S}$ are the diameters of the large and small particles, respectively. This relation is exact for monodisperse particles of homogeneous and equal mass density and provides a good estimate for our slightly polydisperse systems. Table S1 also gives the charge (number) ratios $Z_\mathrm{L}e/(Z_\mathrm{S}e) = Z_\mathrm{L}/Z_\mathrm{S}$, with $Z_\mathrm{L}e$ and $Z_\mathrm{S}e$ the respective charges of the large and small particles. In choosing the particles for the binary mixtures, we exploited our observation that the covalent locking of the steric stabiliser (PHSA-PMMA) molecules to other PMMA chains forming the core of the particle (see Methods) had a profound effect on the particle charge (1). The phase behaviour and electrophoresis measurements indicate that locked particles carry a higher charge than the same particles in the unlocked state.

The values in Table S1 for particles U16, U20, L20 and L29 were taken from (1) and were measured in single-component systems at a volume fraction $\eta \approx 0.01$–$0.02$. As for unlocked particles the surface potential seemed approximately independent of the particle diameter (1), we assumed that the surface potentials of the particles U13 and U29 were similar to the surface potentials of the particles U16 and U20 and used this value to calculate the charge numbers. The charge numbers of the particles in the binary mixtures might have differed from the charge numbers obtained from electrophoresis due to charge regulation, ionic strength, and volume fraction differences.

First, we consider binary systems 1 and 2, which have a mass ratio $m_\mathrm{L}/m_\mathrm{S} = 2.0$. The colloidal Brazil-nut effect is expected for $Z_\mathrm{L}/Z_\mathrm{S} \gtrsim m_\mathrm{L}/m_\mathrm{S}$ (2–4). For system 1, $Z_\mathrm{L}/Z_\mathrm{S} = 1.2$ and the Brazil-nut effect was not observed, in agreement with the predictions from theory and simulations. For system 2, $Z_\mathrm{L}/Z_\mathrm{S}$ varies between 1.9 and 2.8, depending on the sample. The charge ratio was close to that at which the crossover to the Brazil-nut effect is predicted. Note that the crossover value depends on the system parameters, such as the Debye screening length $\kappa^{-1}$, the buoyant masses $m_\mathrm{L}$ and $m_\mathrm{S}$ of the particles (4), and presumably also on the charges $Z_\mathrm{L}$ and $Z_\mathrm{S}$ of the particles. Because the charge ratio was close to the crossover value, only slight changes in the charge ratio would be sufficient to change the system's behaviour from Brazil-nut to non-Brazil-nut at low overall volume fractions around $\eta = 0.02$. Indeed, we found that this system in some cases did and in other cases did not display the Brazil-nut effect, again in agreement with the theory and simulations.

Next, we consider binary systems 3 and 4, both of which have a mass ratio $m_\mathrm{L}/m_\mathrm{S} = 11$. Our estimates for the charge ratio $Z_\mathrm{L}/Z_\mathrm{S}$ are $\sim 4.7$ for system 3 and $\sim 6.4$ for system 4. For the Brazil-nut effect to occur, the ratio $Z_\mathrm{L}/Z_\mathrm{S}$ should be at least 11 (2, 3), but probably larger (4). The observations for systems 3 and 4 (no Brazil-nut effect) are thus also consistent with theory and simulations.

## Characterization of particle charges and correspondence between particle charges and effective charges

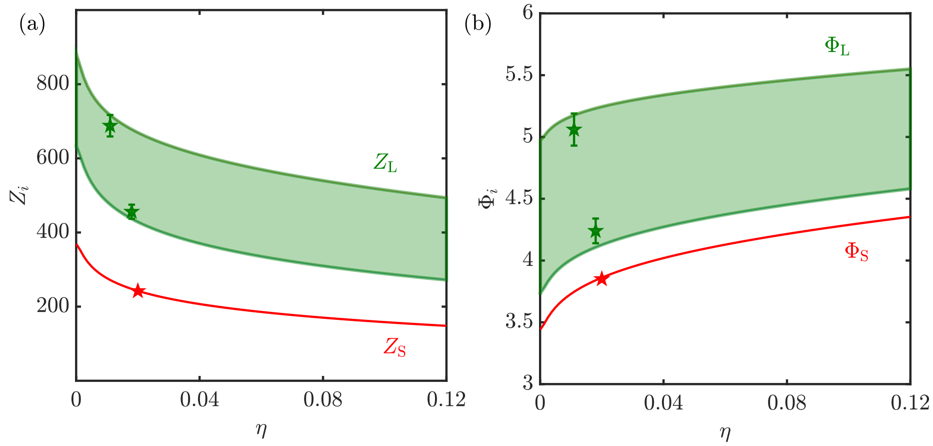


**Fig. S1. Charging of particles in one-component systems.** Based on the electrophoresis measurements in Table S1, we calculate (a) the particle charges $Z_\mathrm{L}$ and $Z_\mathrm{S}$, and (b) the surface potentials $\Phi_\mathrm{L}$ and $\Phi_\mathrm{S}$ as a function of volume fraction $\eta$ using a single-adsorption charge regulation boundary condition within the spherical cell model. The results are valid for homogeneous systems.

From the particle charges of the one-component systems in Table S1, we can estimate the particle charges in the mixture. First, we characterise the charge-regulation parameters in the one-component systems using the cell model. We approximate the colloidal suspension consisting of $N$ spherical cells of radius $R$, each containing a colloidal particle of radius $a$ with charge $Ze$. The cells can overlap, so the volume fraction is given by $\eta = (a/R)^3$. The electrolyte consists of two monovalent ion species, which within the mean-field approximation are described by the ion densities $\rho_\pm(r) = c_\mathrm{s}\exp[\mp\phi(r)]$, with $c_\mathrm{s}$ a given bulk ion concentration of the salt ions. Inserting these densities in the Poisson equation gives the Poisson-Boltzmann equation for a single cell

$$\phi''(r) + \frac{2}{r}\phi'(r) = \kappa^2 \sinh[\phi(r)], \quad r \in (a, R] \qquad [1]$$

with the reservoir screening length $\kappa^{-1} = (8\pi\ell_\mathrm{B}c_\mathrm{s})^{-1/2}$ and $\ell_\mathrm{B}$ is the Bjerrum length. Furthermore, a prime indicates a derivative with respect to $r$. We invoke that each cell is charge neutral, and using the Gauss law around the particle surface gives the boundary conditions

$$\phi'(a) = -\frac{Z\ell_\mathrm{B}}{a^2}, \quad \phi'(R) = 0. \qquad [2]$$

For the particle charge, we assume that only cations can adsorb, using the same model as for the effective charge,

$$Z = \gamma^\mathrm{C} c_\mathrm{s}\exp[-\phi(a)], \qquad [3]$$

with $\gamma^\mathrm{C}$ the cationic chargeability parameter (see main text). We added the superscript C to emphasise that the quantity is associated with the actual particle charge, whereas in the main text, it is associated with the effective charge.

In Fig. S1, we use the data of Ref. (1) to estimate the particle charges and surface potentials of particles L20 and U16 in one-component systems. We used the experimentally determined particle charge to assess the value of $\gamma^\mathrm{C}$ for each of the particles. There is a spread in the estimation of particle charges for the large green particles because there are two independent measurements of the particle charge in which external factors can be changed (e.g., ionic strength). For our estimation, we did not correct this but instead fixed $\kappa^{-1} = 6$ $\mu$m and instead calculated the range in which we expect the particle charges to lie. It should be stressed that this is an estimate based on a very limited number of experimental data points.

In the case of a mixture, we can extend the cell model for the binary case. Such cell models have various realisations depending on how the global charge neutrality condition is invoked. We choose a model where there are two types of cells, there are $N_\mathrm{L}$ cells of the first type contain a large particle with radius $a_\mathrm{L}$, and there are $N_\mathrm{S}$ cells of the second type containing a small particle with radius $a_\mathrm{S}$. Both types of cells have the same radius $R$, such that the volume fraction is $\eta_i = x_i(a_i/R)^3$ with $x_i = N_i/(N_\mathrm{L} + N_\mathrm{S})$ the number fraction for $i =$L,S. For each cell, we have a Poisson-Boltzmann equation again to solve

$$\phi_i''(r) + \frac{2}{r}\phi_i'(r) = \kappa^2 \sinh[\phi_i(r)], \quad r \in (a_i, R], \qquad [4]$$

for $i =$L, S. Within the binary cell model, we invoke global charge neutrality by imposing that the weighted average of all the cells should be charge neutral. Furthermore, there is only one Donnan potential $\Phi_\mathrm{D}/(\beta e)$ common to every cell. We arrive at the set of boundary conditions

$$\phi_i'(a_i) = -\frac{Z_i\ell_\mathrm{B}}{a_i^2}, \quad \sum_{i=\mathrm{L,S}} x_i\phi_i'(R) = 0, \quad \phi_i(R) = \Phi_\mathrm{D}. \qquad [5]$$

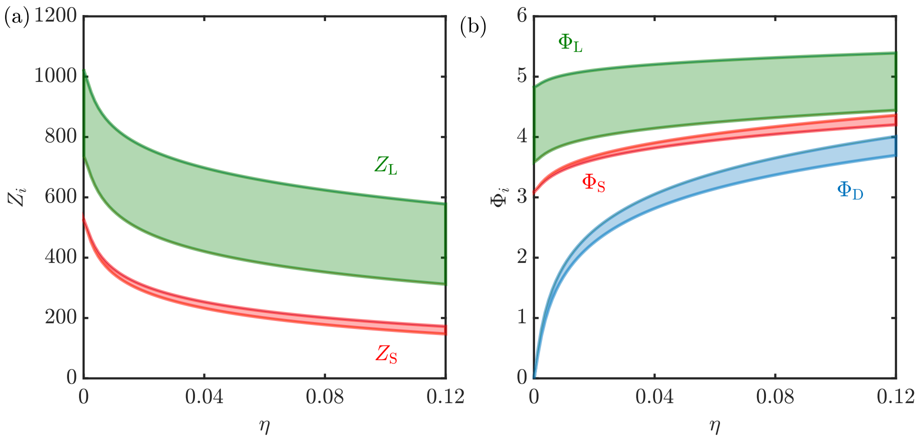


**Fig. S2. Charging of particles in binary mixtures.** (a) Using the same parameters as in Fig. S1 for one-component systems, we estimate the particle charges $Z_{\rm L}$ and $Z_{\rm S}$ as function of the total volume fraction $\eta$ for a 1:1 mixture. (b) The surface potentials $\Phi_{\rm L}$ and $\Phi_{\rm S}$ correspond to the particle charges in (a). Furthermore, we plot the expected range of the Donnan potential $\Phi_{\rm D}$ within the binary cell model.

Note that in this calculation, the Donnan potential should be self-consistently determined. For the charge, we use

$$Z_i = \gamma_i^{\rm C} c_{\rm s} \exp[-\phi_i(a_i)], \qquad [6]$$

Using the estimate of the values for $\gamma_{\rm S}^{\rm C}$ and the upper and lower bound estimate for $\gamma_{\rm L}^{\rm C}$, we calculate using this model the approximate particle charges in a 1:1 binary mixture of particles L20 and U16 as a function of the total volume fraction, see Fig. S2(a). Furthermore, from the same calculation, the surface potentials follow as well as the Donnan potential $\Phi_{\rm D}$, see Fig. S2(b).

This calculation provides a possible link between the particle charges for homogeneous systems and the effective charges used in the main text within the point-charge model. For example, assuming that upon mixing suspensions consisting of particles L20 and U16 that the ionic strength has not yet increased due to the decomposition of the solvent, we can calculate the Donnan potential for a homogenous mixture within the point charge model $\phi_{\rm D}/(\beta e)$ by using the effective charges. We used

$$\phi_{\rm D} = \operatorname{arsinh}\left\{\frac{\sum_i Z_i^0 \bar{\eta}_i/[(\pi/6)\sigma_i^3]}{2c_s}\right\} \qquad [7]$$

which corresponds to Eq. (11) in the main text. Note that $Z_{\rm L,S}^0$ are *effective charges*. Using the parameters to match the sedimentation profiles of total volume fraction $\bar{\eta} = 0.02$ in the main text, we find $\phi_{\rm D} = 2.2$. This value is similar to the $\Phi_{\rm D}$ obtained within the binary cell model using the actual particle charges. For the parameters used to describe the $\bar{\eta} = 0.07$ sample, we find $\phi_{\rm D} = 2.7$, giving again good agreement with the cell model result for $\Phi_{\rm D}$. Therefore, the effective charges used in the main text are expected to reasonably agree with the actual particle charges that are measured with electrophoresis. In the main text, however, we used a smaller value for $\kappa^{-1}$ because we expect that the ionic strength increases over time. This is under the additional assumption that the ions generated in such processes do not contribute to the effective charg

## Additional information on the effects of charge regulation

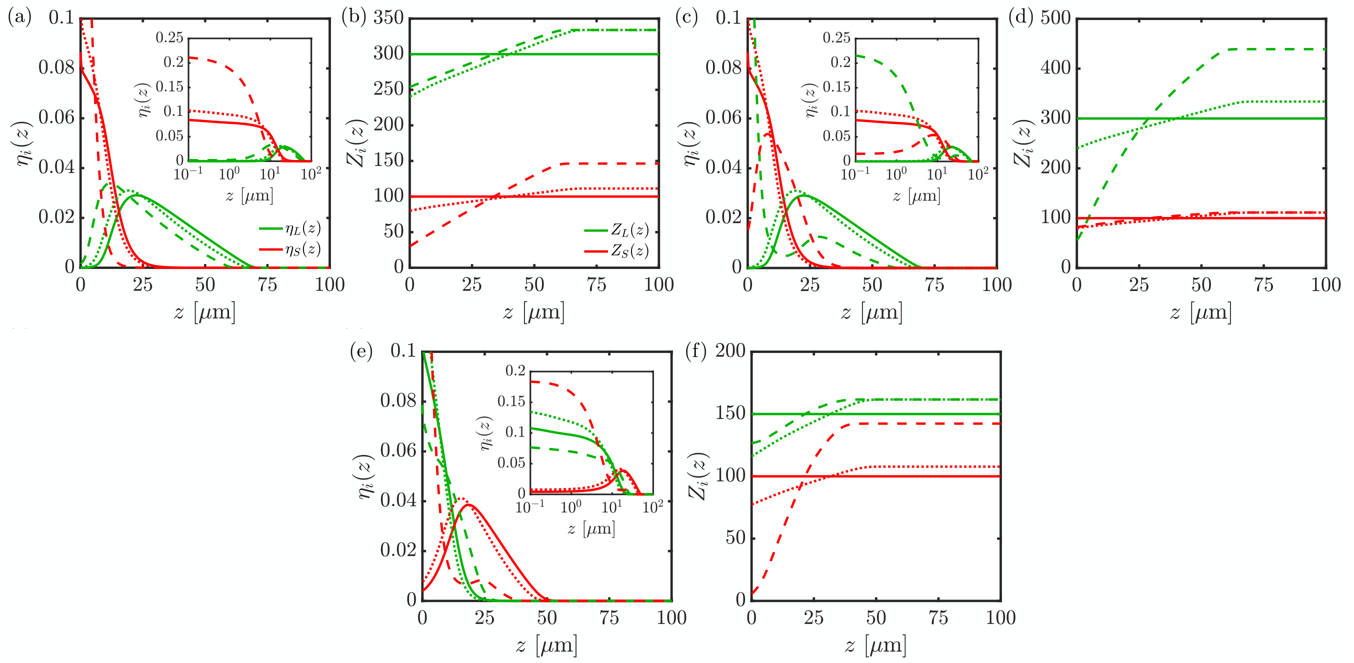


**Fig. S3. Effect of charge regulation on density profiles and local particle charge** (a,c,e) Equilibrium sedimentation profiles with height-dependent packing fractions $\eta_i(z)$ for a binary mixture of charge colloidal particles with and without charge regulation. The inset shows the same plots but in a linear-log scale, highlighting the density inversion that can occur due to charge regulation. (b,d,e) Height-dependent colloidal charge numbers $Z_i(z)$ for small (S) and large particles (L) for the cases (a,c,e), respectively. (a-d) The charge number of the homogeneous mixture are $Z_{\rm L}^0 = 300$, $Z_{\rm S}^0 = 100$, for constant charge (full lines, lines in (a,b) are duplicated in (c,d) for clarity), charge regulation with only adsorption of cations (dotted lines, $\alpha_{\rm S} = \alpha_{\rm L} = 0$, lines from (a,b) are duplicated in (c,d)) and charge regulation where also anions can adsorb, but only on the small particles (dotted line in (a-b), $\alpha_{\rm S} = 0.5$, $\alpha_{\rm L} = 0$), or only on the large particle (dotted line in (c-d), $\alpha_{\rm S} = 0$, $\alpha_{\rm L} = 0.5$). (e-f) Same plots but with lower charge, $Z_{\rm L}^0 = 150$, $Z_{\rm S}^0 = 100$, full lines are again constant charge; dotted lines are charge regulation with only cation adsorption ($\alpha_{\rm S} = \alpha_{\rm L} = 0$). For the dashed lines, small particles can also adsorb anions ($\alpha_{\rm S} = 0.6$, $\alpha_{\rm L} = 0$).

In Fig. S3, we highlight the effects of charge regulation on the density profiles and local particle charge in equilibrium. The non-equilibrium case is discussed in the main text. In all the examples, the large particle (green) has a higher particle charge than the small particle (red) in bulk.

First, we discuss the case where the bulk charges are tuned such that there is a Brazil-nut effect (top row of Fig. S3), and the green particles reside at higher $z$ than the red particles. Fixing bulk charges, rather than equilibrium constants, allows for a straightforward comparison between the various cases. When the particles are charge regulating and acquire their charge purely via cation adsorption (dotted lines), we only see a small difference with the constant-charge case (full lines). Both types of particles acquire a higher density at low $z$ [inset of Fig. S3(a)], and particles discharge for low $z$ because the local density is higher [Fig. S3(b)]. Dotted lines are repeated in Figs. S3(c) and (d).

When also anion adsorption is possible, it is not enough to specify the bulk charges of the particles. In addition, we need to fix the scaled equilibrium constant for anion adsorption $\alpha_i$ ($i = \mathrm{L}, \mathrm{S}$), see Methods. When anions can adsorb a particle, they have a larger tendency to discharge at high local density; this is demonstrated in the dashed lines Figs. S3(b) and (d) for anion adsorption on the small and large particle only, respectively. Indeed, the local charge ratio between large and small particles increases for $\alpha_{\rm L} \neq 0$ [Fig. S3(b)], whereas it becomes smaller for $\alpha_{\rm S} \neq 0$ [Fig. S3(d)]. Furthermore, anion adsorption changes the shape of the density profile for the particle that resides at larger $z$ [Fig. S3(c)] if it is allowed to adsorb anions. This shape change is associated with a change of the local charge ratio at sufficiently low $z$, so the condition for the Brazil-nut effect to occur is violated locally.

Finally, similar effects occur when there is no Brazil-nut effect (bottom row of Fig. S3). Charge regulating particles with cation adsorption only differ quantitatively in density profiles from the constant-charge case S3(e) at low $z$. Anion adsorption can drastically change the shape of the profile when it occurs on the particle residing at larger $z$.

The effects of charge regulation in equilibrium are summarised in Fig. S4. Here we take $m_{\rm L}/m_{\rm S} = 2$. For constant-charge particles, a Brazil-nut effect occurs in equilibrium when $Z_{\rm L}^0/Z_{\rm S}^0 > m_{\rm L}/m_{\rm S}$, and this is indeed observed if we probe the mean height as a function of the charge ratio, full lines in Fig. S4a. When both particles are charge regulating but with only cation adsorption allowed, the mean heights are altered for a fixed bulk charge ratio. Still, the transition to a Brazil-nut effect occurs approximately at the same charge ratio as the constant-charge case. When anion adsorption is included, one can either suppress the Brazil-nut effect or induce the Brazil-nut effect compared to what is expected on the charge ratio of the homogeneous mixture. In Fig. S4b, we show that anion adsorption on the large particle with lower charge can locally decrease

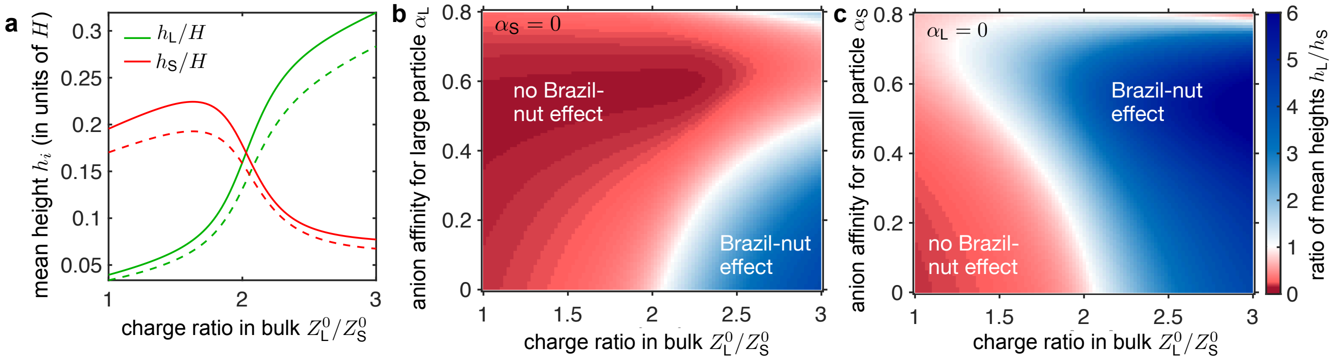


**Fig. S4. Effect of charge regulation on the occurrence of the Brazil-nut effect in equilibrium** **a** Mean heights $h_i$ for small (S) and large (L) particles concerning the sample cell height $H$, as a function of the charge ratio $Z_L^0/Z_S^0$ of the homogeneous mixture for constant charge (full lines) and charge regulation with cation adsorption only (dashed lines, $\alpha_L = \alpha_S = 0$). **b** State diagram of the colloidal Brazil nut effect (Brazil-nut effect, occurs for $h_L/h_S > 1$) as a function of the tendency for anion adsorption on the large particle, as quantified by $\alpha_L$, but when no anions can adsorb on the small particle ($\alpha_S = 0$). **c** Same as in **b**, but now as a function of the anion adsorption tendency on the small particle, controllable by the parameter $\alpha_S$, and no anion adsorption on the large particle ($\alpha_L = 0$). In all plots $Z_S^0 = 100$, Debye screening length $\kappa^{-1} = 1$ $\mu$m, volume fractions of the homogeneous mixture $\bar{\eta}_L = \bar{\eta}_S = 0.01$, and other parameters are the same as the ones from the experiment, see main text.

the charge ratio and therefore suppress the Brazil-nut effect for $Z_L^0/Z_S^0 > m_L/m_S$. In contrast, when there is anion adsorption on only the small particle, locally, the charge ratio can increase, therefore inducing the Brazil-nut effect for low charge ratios $Z_L^0/Z_S^0 < m_L/m_S$, see Fig. S4c.

Finally, note that the shape of the density profile is also important for the mean height: the particle species that can adsorb anions sometimes has a non-monotonous density profile, with a local maximum that becomes more pronounced for larger anion affinity. This can again increase the mean height of this particular particle species, which explains the "re-entrant" behaviour of (no) Brazil-nut effect in Figs. S4(b-c) for higher ($\alpha_L$) $\alpha_S$, at sufficiently (high) low $Z_L^0/Z_S^0$.

## Effects of unequal diffusion constants

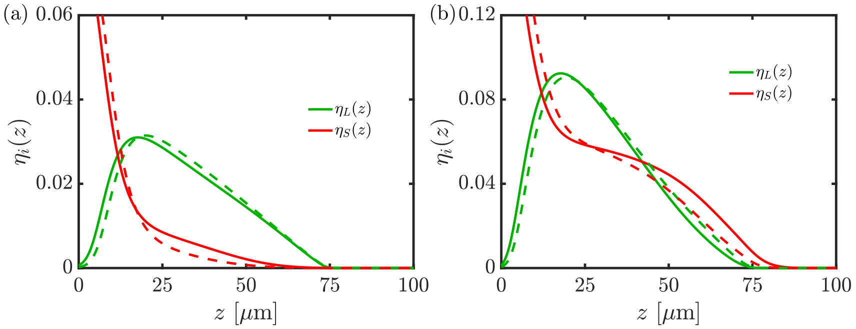


**Fig. S5. Influence of not equal diffusion coefficients.** We replotted the theoretical prediction for the experimental data for (a) the $\bar{\eta} = 0.02$ sample and (b) the $\bar{\eta} = 0.07$ sample as the solid lines, assuming an equal diffusion coefficient for large and small particles. The same data can be found in Fig. 2 (main text, solid lines). As dashed lines, we plot the results when we take the diffusion coefficients to be unequal, approximating the ratio of diffusion coefficients by the Stokes drag formula and invoking the fluctuation-dissipation theorem.

In the main text, we made two main assumptions regarding the collective diffusion coefficients of the charged colloidal particles. (i) We neglected hydrodynamic interactions such that the diffusion constants are effectively that of a single particle. (ii) We assumed an equal diffusion coefficient for the charged colloidal particles to reduce the number of fitting parameters. Therefore, this could be a limiting assumption. Here, we will relax condition (ii) to investigate an unequal diffusion constant of the particles. We use the large particle to set the time scale of diffusion, i.e.

$$\tau_{\mathrm{D}} = \frac{\sigma_{\mathrm{L}}^2}{4D_{\mathrm{L}}}. \qquad [8]$$

We do not attempt to determine the single particle diffusion constant $D_{\mathrm{L}}$ like in the main text. However, we can approximate the ratio between the diffusion constants of large and small particles. This ratio within the Stokes-Einstein approximation is $D_{\mathrm{S}}/D_{\mathrm{L}} = \sigma_{\mathrm{L}}/\sigma_{\mathrm{S}} = 1.25$ for the particles L20 and U16 used in the main text. Using this result, we recalculated the density profiles describing the experimental data in the main text, keeping all other model parameters fixed, see Fig. S5, dashed lines. An unequal diffusion constant changes the density profiles slightly quantitatively but does not change the shape compared to the equal-constant approximation. Therefore, we are confident that the equal-diffusion constant model in the main text is justified.

**Movie S1. Sedimentation profile in a binary suspension of large (green) and small (red) particles at an overall volume fraction of 0.02. Particles sediment towards the top wall. This sample exhibits the colloidal Brazil-nut effect. Video shows a stack of *xy* confocal microscopy images, as viewed when starting at the top wall and moving downwards. Video corresponds to sample 2 in Table S1. The density profile is shown in Fig. 3a.**

**Movie S2. Sedimentation profile in a binary suspension of large (green) and small (red) particles at an overall volume fraction of 0.07. Particles sediment towards the top wall. This sample does not exhibit the colloidal Brazil-nut effect. Video shows a stack of *xy* confocal microscopy images, as viewed when starting at the top wall and moving downwards. Video corresponds to sample 2 in Table S1. The density profile is shown in Fig. 3b.**

## References


1. MN van der Linden, et al., Charging of poly(methyl methacrylate) (pmma) colloids in cyclohexyl bromide: Locking, size dependence, and particle mixtures. *Langmuir* **31**, 65–75 (2015).
2. A Esztermann, H Löwen, Colloidal Brazil-nut effect in sediments of binary charged suspensions. *Eur. Lett.* **68**, 120–126 (2004).
3. J Zwanikken, R van Roij, The sediment of mixtures of charged colloids: segregation and inhomogeneous electric fields. *Eur. Lett.* **71**, 480–486 (2005).
4. M Dijkstra, J Zwanikken, R van Roij, Sedimentation of binary mixtures of like- and oppositely charged colloids: the primitive model or effective pair potentials? *J. Phys.: Condens. Matter* **18**, 825–836 (2006).
